# Supplementary material for: Robust Multicovers with Budgeted Uncertainty
Source: arXiv:1812.04622 source file (2018-12-13)
Supplement: Supplementary file 1 [file appendix_tables.tex]

This section contains the exact results of our computations. 
The keyword \emph{DNF} (``did not finish'') in this case means that the according approach was not able to solve the instance within the given total time limit (wall clock time). The times are rounded to the second position after decimal point. 

\subsection{Random Instances}
\label{appendix:random}
The average objective values of the random instances are rounded to the second position after decimal point. For the random instances, we use a total time limit of two minutes. Further, note that average processing times are displayed.

%% [inline block 0: 1 envs, 73479 chars -> data_tex | \begin{tabular}{|c|c|c|c|c|c|c|c|c|c|>{\centering\arraybackslash}p{1.7cm}|c|} ...]

%\caption{Results for real world instances with $irt=2$.}
%\label{table:irt2}
%\end{table}
